# Supplementary material for: Jointly constrained semidefinite bilinear programming with an application to Dobrushin curves
Source: arXiv:1808.03182 ancillary file (2018-08-09)
Supplement: Supplementary file 1 [file documentation.pdf]

# Jointly constrained semidefinite bilinear programming with an application to Dobrushin curves - Python Code

Stefan Huber, Robert König and Marco Tomamichel

August 9, 2018

The code consists of the following files:

```
anc/
├── tree.py
├── problem.py
├── bilinear.py
├── examples/
│   ├── ex_tracedist.py
│   └── ex_dobrushin.py
```

The file `tree.py` contains the definition of the `tree` class, which is the main data structure used for the algorithm. The file `problem.py` implements a solver for bilinear problems, and the file `semidefinite.py` defines the `QuantumBilinearProblem` class, which is the class with which the user interacts. The folder `examples` contains two working examples of the applications we explain below.

We give some examples to show the usage of the `QuantumBilinearProblem` class.

We assume the following header for all code:

```
from semidefinite import *
from problem import *
import numpy as np
import picos as sdp
import cvxopt as cvx
```

In general, an instance of `QuantumBilinearProblem`, which we call `prob`, is created via

```
prob = QuantumBilinearProblem()
```

Then we can initialize the problem by giving the correlation matrices and affine terms (corresponding to  $Q$ ,  $A$ ,  $B$  in the objective function  $f(X, Y) = \text{tr}((X \otimes Y)Q) + \text{tr}(AX) + \text{tr}(BY)$ ):

```
prob.init_matrix_form(dims, J, A = [], B = [])
```

The syntax for `dims` is  $[[a_1, a_2, \dots, a_r], [b_1, b_2, \dots, b_s]]$ . Here, the variables  $X = X_1 \oplus \dots \oplus X_r$  and  $Y = Y_1 \oplus \dots \oplus Y_s$  are interpreted as being self-adjoint operators in Hilbert spaces which are direct sums of

qudits  $\mathbb{C}^{a_1} \oplus \dots \oplus \mathbb{C}^{a_r}$  and  $\mathbb{C}^{b_1} \oplus \dots \oplus \mathbb{C}^{b_s}$ , respectively. In our implementation, all  $a_i$  and  $b_j$  need to be powers of 2 (in the implementation, we have chosen the Pauli basis and direct sums thereof). It is straightforward to generalize this to qudit systems of arbitrary dimensions by choosing a different basis. The input  $J$  is an array of the form  $r \times s$  where every entry  $J_{ij}$  is an  $a_i b_j \times a_i b_j$  matrix which defines the correlations between the  $i$ -th  $X$ -variable and the  $j$ -th  $Y$ -variable. Furthermore,  $A$  and  $B$  are arrays of length  $r$  and  $s$ , respectively, such that  $A_i$  defines the affine term in the variable  $X_i$  and  $B_i$  defines the affine term in the variable  $Y_i$ . That is, the objective function is

$$f(X, Y) = \sum_{i=1}^r \sum_{j=1}^s \text{tr}(J_{ij}(X_i \otimes Y_j)) + \sum_{i=1}^r \text{tr}(X_i A_i) + \sum_{j=1}^s \text{tr}(Y_j B_j) .$$

We will demonstrate this in a concrete example.

Constraints can be added by the routine `add_constraint`. Say  $X = X_1 \oplus \dots \oplus X_r$ , and we want to add the constraint  $0 \leq X_j \leq I$ . This can be done by adding a constraint on `prob.matvarX(j)`, which is the matrix form of  $X_j$ . `prob.matvarY(j)` is defined analogously.

```
prob.add_constraint(prob.matvarX(j) >= 0.*np.identity(a_j))
prob.add_constraint(prob.matvarX(j) <= np.identity(a_j))
```

Trace constraints can be added similarly, by using the routine `add_constraint` to add constraints on the entries of `prob.varX()`, which is an array containing the coordinates of  $X_1$  with respect to the Pauli basis, followed by the coordinates  $X_2$  with respect to the Pauli basis, and so on. The array `prob.varY()` is defined analogously. As an example, consider the case  $b_1 = 2, b_2 = 2$ , and we want to add the constraints  $\text{tr}(Y_1 \sigma_3) \leq E$  and  $\text{tr}(Y_2) = 1$ . This can be done via

```
prob.add_constraints(prob.varY()[3] == E/np.sqrt(2))
prob.add_constraints(prob.varY()[4] == 1/np.sqrt(2))
```

Note that we need to add a factor of  $\sqrt{2}$  because we worked with the Pauli basis normalized with respect to the Hilbert-Schmidt inner product.

Finally, the branch-and-bound algorithm to solve the problem can be started by the line

```
prob.solve(verb = 1, maxiter = STD_MAXITER, allowedgap = STD_ALLOWEDGAP)
```

The standard values of `maxiter` and `allowedgap` are  $10^5$  and  $10^{-5}$ , respectively. After the algorithm has finished running, we can call the solutions via `prob.matsolX(j)` and `prob.matsolY(j)`.

## Example: A simple trace distance maximization

Consider the problem

$$\max_{\substack{X, Y \geq 0 \\ \text{tr}(X) = \text{tr}(Y) = 1}} \|X - Y\|_1 = \max_{\substack{X, Y \geq 0 \\ \text{tr}(X) = \text{tr}(Y) = 1}} \max_{\substack{P \in \mathcal{B}_{\text{sa}}(\mathbb{C}^2) \\ 0 \leq P \leq I}} \text{tr}(P(X - Y)) .$$

Note that using the flip operator  $\mathbb{F} = \sum_{i,j=1}^2 |ij\rangle\langle ji|$ , we can write the objective function in the form

$$\text{tr}(\mathbb{F}(X \otimes P)) - \text{tr}(\mathbb{F}(Y \otimes P)) .$$

It is easy to see that this can also be written as a minimization problem, namely

$$- \min_{\substack{X, Y, P \geq 0 \\ \text{tr}(X) = \text{tr}(Y) = 1 \\ 0 \leq P \leq I}} \text{tr}(\mathbb{F}(X \otimes P)) - \text{tr}(\mathbb{F}(Y \otimes P)) .$$

We interpret the variables as follows: `matvarX(0)` plays the role of  $X$ , `matvarX(1)` plays the role of  $Y$ , and `matvarY(0)` plays the role of  $P$ . Hence  $a_1 = a_2 = b_1 = 2$ , and this problem can be solved in the following way:

```

prob = QuantumBilinearProblem()
flip = np.matrix([[1.,0.,0.,0.], [0.,0.,1.,0.], [0.,1.,0.,0.], [0.,0.,0.,1.]])

prob.init_matrix_form([[2, 2], [2]], [[-flip], [flip]])

prob.add_constraint(prob.matvarX(0) >> 0*np.identity(2))
prob.add_constraint(prob.matvarX(1) >> 0*np.identity(2))
prob.add_constraint(prob.matvarY(0) >> 0*np.identity(2))
prob.add_constraint(prob.matvarY(0) << np.identity(2))

prob.add_constraint(prob.varX()[0] == 1./np.sqrt(2))
prob.add_constraint(prob.varX()[4] == 1./np.sqrt(2))

prob.solve(verb = 1)

print('X = ', prob.matsolX(0))
print('Y = ', prob.matsolX(1))
print('P = ', prob.matsolY(0))

```

The file `examples/ex_tracedist.py` contains the full code which implements this problem.

## Example: Computing a qubit Dobrushin curve

As a second example, we show how to compute a point on the Dobrushin curve of a dephasing channel. We recall that this problem is given by

$$F_E(\delta) = \delta \max_{(P,Q,R) \in \Gamma(E,\delta)} \text{tr}(P\Phi(2R - I)) ,$$

where  $\Gamma(E, \delta)$  is the set of triples  $(P, Q, R) \in \mathcal{B}(\mathbb{C}^2)^{\times 3}$  satisfying

$$\begin{aligned}
& \text{tr}(Q) = 1, Q \geq 0, \text{tr}(HQ) \leq E , \\
& Q + \frac{\delta}{2}(2R - I) \geq 0 , \\
& \text{tr}(H(Q + \frac{\delta}{2}(2R - I))) \leq E , \\
& \text{tr}(R) = 1 , \\
& 0 \leq R , \\
& 0 \leq P \leq I , \\
& \text{tr}(P) = 1 .
\end{aligned}$$

We also recall that the objective function can be recast as

$$\text{tr}(P\Phi(2R - I)) = 2 \text{tr}((I \otimes \Phi^*)(\mathbb{F})(P \otimes R)) - \text{tr}(P\Phi(I)) .$$

In the code here, `matvarX(0)` plays the role of  $R$ , `matvarX(1)` plays the role of  $Q$ , and `matvarY(0)` plays the role of  $P$ . For fixed values of  $\delta$  and  $E$ , which we call `delt` and `E` in the program, we can solve this problem by the following code:

```

prob = QuantumBilinearProblem()

corr = np.matrix([[1.,0.,0.,0.], [0.,0.,1/2.,0.], [0.,1/2.,0.,0.], [0.,0.,0.,1.]])

prob.init_matrix_form([[2, 2], [2]], [[2.*delt*corr], [0.*corr]],
    A = [], B = [-1.*delt*np.identity(2)])

prob.add_constraint(prob.matvarX(0) >> 0*np.identity(2))
prob.add_constraint(prob.matvarX(1) >> 0*np.identity(2))
prob.add_constraint(prob.matvarX(0) << np.identity(2))
prob.add_constraint(prob.matvarX(1) + delt*prob.matvarX(0) >> delt/2.*np.identity(2))
prob.add_constraint(prob.matvarY(0) >> 0*np.identity(2))
prob.add_constraint(prob.matvarY(0) << np.identity(2))

prob.add_constraint(prob.varX()[0] == 1./np.sqrt(2.))
prob.add_constraint(prob.varX()[4] == 1./np.sqrt(2.))
prob.add_constraint(prob.varX()[7] == E/np.sqrt(2.))
prob.add_constraint(prob.varX()[7] + delt*prob.varX()[3] == E/np.sqrt(2.))
prob.add_constraint(prob.varY()[0] == 1./np.sqrt(2.))

prob.solve(verb = 1)

```

The file `examples/ex_dobrushin.py` contains the full code which implements this problem.
